# Supplementary material for: Enhancing Intrinsic Features for Debiasing via Investigating Class-Discerning Common Attributes in Bias-Contrastive Pair
Source: arXiv:2404.19250 source file (2024-06-17)
Supplement: Supplementary file 1 [file dataset.tex]

\begin{table*}[h!]
\centering
\resizebox{0.8\linewidth}{!}{
\setlength{\tabcolsep}{1.0em}
\begin{tabular}{ c | c c | c c | c c }
% \hline\noalign{\smallskip}
\toprule

% \\ \midrule
% \multicolumn{3}{c}{}
\multirow{2}{*}{Ratio (\%)} & \multicolumn{2}{c}{Waterbirds} & \multicolumn{2}{c}{BFFHQ} & \multicolumn{2}{c}{BAR} \\
\cmidrule(lr){2-3}\cmidrule(lr){4-5}\cmidrule(lr){6-7} 
                        & \# BA & \# BC  & \# BA & \# BC & \# BA & \# BC \\
\midrule
        0.5 & 4771 & 24   & 19104 & 96  & N/A & N/A\\
        1.0 & 4747 & 48   & 19008 & 192 & N/A & N/A\\
        2.0 & 4699 & 96   & 18816 & 384 & N/A & N/A\\
        5.0 & 4555 & 240  & 18240 & 960 & N/A & N/A\\

\bottomrule
\end{tabular}}
% \vspace{-0.5cm}
\caption{The number of bias-aligned samples (\# BA samples) and bias-conflicting ones~(\# BC samples) in training datasets. }
\label{tab:supp_data}
\end{table*}
