# Supplementary material for: Enhancing Intrinsic Features for Debiasing via Investigating Class-Discerning Common Attributes in Bias-Contrastive Pair
Source: arXiv:2404.19250 source file (2024-06-17)
Supplement: Supplementary file 2 [file recentwork_comparison.tex]

% \begin{table}[t!]
% \centering
% \resizebox{1\linewidth}{!}{
% \setlength{\tabcolsep}{0.7em}
% \def\arraystretch{0.9}% 
% \begin{tabular}{ l | c c c c | c c}
% \toprule 

% \multicolumn{1}{c|}{\multirow{2}{*}{}}

% & \multicolumn{4}{c|}{BFFHQ}  
% & \multicolumn{2}{c}{BAR} 

% \\ \cmidrule(lr){2-5} \cmidrule(lr){6-7} 

% BS
% & 0.5\% 
% & 1.0\%
% & 2.0\%
% & 5.0\%
% & 1.0\%
% & 5.0\%

% \\
% \midrule

% DCWP~\cite{dcwp2023park}
% & 64.08 & 67.44 & 75.24 & 85.00 & 69.63 & 81.79 \\ % (no imagenet)
% Ours
% & \textbf{71.68} & \textbf{77.56} & \textbf{83.08} & \textbf{87.60} & \textbf{75.14} & \textbf{85.03} \\

% \bottomrule
% \end{tabular}}
% \caption{Comparison with the DCWP. BS is bias severity}
% \label{tab:recent_comparison}
% \end{table}

\begin{table*}[t!]
\centering
\resizebox{0.8\linewidth}{!}{
\setlength{\tabcolsep}{1.0em}
\begin{tabular}{ l | c c c c | c c}
\toprule 

\multicolumn{1}{c|}{\multirow{2}{*}{}}

& \multicolumn{4}{c|}{BFFHQ}  
& \multicolumn{2}{c}{BAR} 

\\ \cmidrule(lr){2-5} \cmidrule(lr){6-7} 

BS
& 0.5\% 
& 1.0\%
& 2.0\%
& 5.0\%
& 1.0\%
& 5.0\%

\\
\midrule

DCWP~\cite{dcwp2023park}
& 64.08\stdv{0.00} & 67.44\stdv{0.00} & 75.24\stdv{0.00} & 85.00\stdv{0.00} & 69.63\stdv{0.00} & 81.79\stdv{0.00} \\ % (no imagenet)
Ours
& \textbf{71.68}\stdv{0.00} & \textbf{77.56}\stdv{0.00} & \textbf{83.08}\stdv{0.00} & \textbf{87.60}\stdv{0.00} & \textbf{75.14}\stdv{0.00} & \textbf{85.03}\stdv{0.00} \\

\bottomrule
\end{tabular}}
\caption{Comparison with the DCWP. BS is bias severity}
\label{tab:recent_comparison}
\end{table*}
